# Supplementary material for: MEMC-Net: Motion Estimation and Motion Compensation Driven Neural Network for Video Interpolation and Enhancement
Source: arXiv:1810.08768 source file (2019-09-05)
Supplement: Supplementary file 1 [file MiddleburyEvaluation.tex]

\begin{figure}[!h]
	\vspace{-0.2cm}
	%	\footnotesize
	\footnotesize
%	\tiny
	\centering
	 % adjust horizontal space
	 % adjust vertical space
\begin{center}
	\begin{tabular}{cc}
\includegraphics[width=0.49\linewidth]{supp/MiddleburySet/eval-result-author/67599_overlay/Dumptruck/frame10i11_IENone_PSNRNone.png}&
\includegraphics[width=0.49\linewidth]{supp/MiddleburySet/eval-result-author/epicflow/Dumptruck/frame10i11_IENone_PSNRNone.png}\\
			(a) Overlay&
			(b) EpicFlow~\cite{revaud2015epicflow}\\
\includegraphics[width=0.49\linewidth]{supp/MiddleburySet/eval-result-author/spynet/Dumptruck/frame10i11_IENone_PSNRNone.png}&
\includegraphics[width=0.49\linewidth]{supp/MiddleburySet/eval-result-author/33758-lf/Dumptruck/frame10i11_IENone_PSNRNone.png}\\
			(c) SPyNet~\cite{ranjan2017optical}&
			(d) SepConv-$L_f$~\cite{niklaus2017videoSepConv}\\
\includegraphics[width=0.49\linewidth]{supp/MiddleburySet/eval-result-author/93785-l1/Dumptruck/frame10i11_IENone_PSNRNone.png}&
\includegraphics[width=0.49\linewidth]{supp/MiddleburySet/eval-result-author/46043_Ours_by12661/Dumptruck/frame10i11_IENone_PSNRNone.png} \\			 
			 (e) SepConv-$L_1$~\cite{niklaus2017videoSepConv}&
			 (f) Ours\\
		\end{tabular}
	\end{center}
	\vspace{-0.5cm}
	\caption{
	\textbf{Visual comparisons on the Middlebury~\cite{baker2011database} \textsc{Evaluation} set. }
	%
%	The sequence is from the \textsc{Evaluation} set. 
	%
	Our method reconstructs a straight and complete lamppost, while existing approaches cannot reconstruct the lamppost well.
	}
\label{fig:MiddleburyDumptruck} %% label for entire figure
\end{figure}

\begin{figure}[!h]
	%	\footnotesize
	\footnotesize
	%	\tiny
	\centering
	 % adjust horizontal space
	 % adjust vertical space
	\begin{center}
		\begin{tabular}{cc}
			\includegraphics[width=0.49\linewidth]{supp/MiddleburySet/eval-result-author/67599_overlay/Backyard/frame10i11_IENone_PSNRNone.png}&
			\includegraphics[width=0.49\linewidth]{supp/MiddleburySet/eval-result-author/epicflow/Backyard/frame10i11_IENone_PSNRNone.png}\\
			(a) Overlay&
			(b) EpicFlow~\cite{revaud2015epicflow}\\
			\includegraphics[width=0.49\linewidth]{supp/MiddleburySet/eval-result-author/spynet/Backyard/frame10i11_IENone_PSNRNone.png}&
			\includegraphics[width=0.49\linewidth]{supp/MiddleburySet/eval-result-author/33758-lf/Backyard/frame10i11_IENone_PSNRNone.png}\\
			(c) SPyNet~\cite{ranjan2017optical}&
			(d) SepConv-$L_f$~\cite{niklaus2017videoSepConv}\\
			\includegraphics[width=0.49\linewidth]{supp/MiddleburySet/eval-result-author/93785-l1/Backyard/frame10i11_IENone_PSNRNone.png}&
			\includegraphics[width=0.49\linewidth]{supp/MiddleburySet/eval-result-author/46043_Ours_by12661/Backyard/frame10i11_IENone_PSNRNone.png} \\			 
			(e) SepConv-$L_1$~\cite{niklaus2017videoSepConv}&
			(f) Ours\\
		\end{tabular}
	\end{center}
	\vspace{-0.1cm}
	\caption{
		\textbf{Visual comparisons on the Middlebury~\cite{baker2011database} \textsc{Evaluation} set.}
		%
%		The sequence is from the \textsc{Evaluation} set.
		%
		The proposed method reconstructs the falling ball with a clear shape and generates fewer artifacts on the foot.
		}
	\label{fig:MiddleburyBackyard} %% label for entire figure
\end{figure}

\begin{figure}[!h]
	%	\footnotesize
	\footnotesize
	%	\tiny
	\centering
	 % adjust horizontal space
	 % adjust vertical space
	\begin{center}
		\begin{tabular}{cc}
			\includegraphics[width=0.49\linewidth]{supp/MiddleburySet/eval-result-author/67599_overlay/Basketball/frame10i11_IENone_PSNRNone.png}&
			\includegraphics[width=0.49\linewidth]{supp/MiddleburySet/eval-result-author/epicflow/Basketball/frame10i11_IENone_PSNRNone.png}\\
			(a) Overlay&
			(b) EpicFlow~\cite{revaud2015epicflow}\\
			\includegraphics[width=0.49\linewidth]{supp/MiddleburySet/eval-result-author/spynet/Basketball/frame10i11_IENone_PSNRNone.png}&
			\includegraphics[width=0.49\linewidth]{supp/MiddleburySet/eval-result-author/33758-lf/Basketball/frame10i11_IENone_PSNRNone.png}\\
			(c) SPyNet~\cite{ranjan2017optical}&
			(d) SepConv-$L_f$~\cite{niklaus2017videoSepConv}\\
			\includegraphics[width=0.49\linewidth]{supp/MiddleburySet/eval-result-author/93785-l1/Basketball/frame10i11_IENone_PSNRNone.png}&
			\includegraphics[width=0.49\linewidth]{supp/MiddleburySet/eval-result-author/46043_Ours_by12661/Basketball/frame10i11_IENone_PSNRNone.png} \\			 
			(e) SepConv-$L_1$~\cite{niklaus2017videoSepConv}&
			(f) Ours\\
		\end{tabular}
	\end{center}
	\vspace{-0.1cm}
	\caption{
		\textbf{Visual comparisons on the Middlebury~\cite{baker2011database} \textsc{Evaluation} set.}
		%
%		The sequence is from the \textsc{Evaluation} set.
		%
        Our method preserves the fine textures of the basketball well and does not produce blockiness or ghost effect.
	}
	\label{fig:MiddleburyBasketball} %% label for entire figure
\end{figure}

\begin{figure}[!h]
	%	\footnotesize
	\footnotesize
	%	\tiny
	\centering
	 % adjust horizontal space
	 % adjust vertical space
	\begin{center}
		\begin{tabular}{cc}
			\includegraphics[width=0.49\linewidth]{supp/MiddleburySet/eval-result-author/67599_overlay/Evergreen/frame10i11_IENone_PSNRNone.png}&
			\includegraphics[width=0.49\linewidth]{supp/MiddleburySet/eval-result-author/epicflow/Evergreen/frame10i11_IENone_PSNRNone.png}\\
			(a) Overlay&
			(b) EpicFlow~\cite{revaud2015epicflow}\\
			\includegraphics[width=0.49\linewidth]{supp/MiddleburySet/eval-result-author/spynet/Evergreen/frame10i11_IENone_PSNRNone.png}&
			\includegraphics[width=0.49\linewidth]{supp/MiddleburySet/eval-result-author/33758-lf/Evergreen/frame10i11_IENone_PSNRNone.png}\\
			(c) SPyNet~\cite{ranjan2017optical}&
			(d) SepConv-$L_f$~\cite{niklaus2017videoSepConv}\\
			\includegraphics[width=0.49\linewidth]{supp/MiddleburySet/eval-result-author/93785-l1/Evergreen/frame10i11_IENone_PSNRNone.png}&
			\includegraphics[width=0.49\linewidth]{supp/MiddleburySet/eval-result-author/46043_Ours_by12661/Evergreen/frame10i11_IENone_PSNRNone.png} \\			 
			(e) SepConv-$L_1$~\cite{niklaus2017videoSepConv}&
			(f) Ours\\
		\end{tabular}
	\end{center}
	\vspace{-0.1cm}
	\caption{
		\textbf{Visual comparisons on the Middlebury~\cite{baker2011database} \textsc{Evaluation} set.}
		%
%		The sequence is from the \textsc{Evaluation} set.
		%
		Our method generates favorable results in the highly textured region. 
	}
	\label{fig:MiddleburyEvergreen} %% label for entire figure
\end{figure}

%
%
%\begin{figure}[!h]
%	%	\footnotesize
%	\footnotesize
%	%	\tiny
%	\centering
%	\renewcommand{\tabcolsep}{1pt} % adjust horizontal space
%	\renewcommand{\arraystretch}{1} % adjust vertical space
%	\begin{center}
%		\begin{tabular}{cc}
%			\includegraphics[width=0.49\linewidth]{supp/MiddleburySet/eval-result-author/67599_overlay/Urban/frame10i11_IENone_PSNRNone.png}&
%			\includegraphics[width=0.49\linewidth]{supp/MiddleburySet/eval-result-author/epicflow/Urban/frame10i11_IENone_PSNRNone.png}\\
%			(a) Overlay&
%			(b) EpicFlow~\cite{revaud2015epicflow}\\
%			\includegraphics[width=0.49\linewidth]{supp/MiddleburySet/eval-result-author/spynet/Urban/frame10i11_IENone_PSNRNone.png}&
%			\includegraphics[width=0.49\linewidth]{supp/MiddleburySet/eval-result-author/33758-lf/Urban/frame10i11_IENone_PSNRNone.png}\\
%			(c) SPyNet~\cite{ranjan2017optical}&
%			(d) SepConv-$L_f$~\cite{niklaus2017videoSepConv}\\
%			\includegraphics[width=0.49\linewidth]{supp/MiddleburySet/eval-result-author/93785-l1/Urban/frame10i11_IENone_PSNRNone.png}&
%			\includegraphics[width=0.49\linewidth]{supp/MiddleburySet/eval-result-author/46043_Ours_by12661/Urban/frame10i11_IENone_PSNRNone.png} \\			 
%			(e) SepConv-$L_1$~\cite{niklaus2017videoSepConv}&
%			(f) Ours\\
%		\end{tabular}
%	\end{center}
%	\vspace{-0.1cm}
%	\caption{
%		\textbf{Visual comparisons on Middlebury~\cite{baker2011database}'s \textsc{Evaluation} set.}
%		%
%%		The sequence is from the \textsc{Evaluation} set.
%		%
%%		Our method is 
%	}
%	\label{fig:MiddleburyUrban} %% label for entire figure
%\end{figure}
