# Supplementary material for: MEMC-Net: Motion Estimation and Motion Compensation Driven Neural Network for Video Interpolation and Enhancement
Source: arXiv:1810.08768 source file (2019-09-05)
Supplement: Supplementary file 2 [file MiddleburyOther.tex]

\begin{figure}[t]
	%	\footnotesize
	\footnotesize
%	\tiny
	\centering
	 % adjust horizontal space
	 % adjust vertical space
\begin{center}
	\begin{tabular}{cc}
\includegraphics[width=0.45\linewidth]{supp/MiddleburySet/other-result-author/MIND/Beanbags/frame10i11_IE1.9268_PSNR29.2371.png}&
\includegraphics[width=0.45\linewidth]{supp/MiddleburySet/other-result-author/demo_outputMB_toflow/Beanbags/frame10i11_IE1.5667_PSNR28.1681.png}\\
			(a) MIND~\cite{long2016learning}&
			(b) ToFlow~\cite{xue2017video}\\

\includegraphics[width=0.45\linewidth]{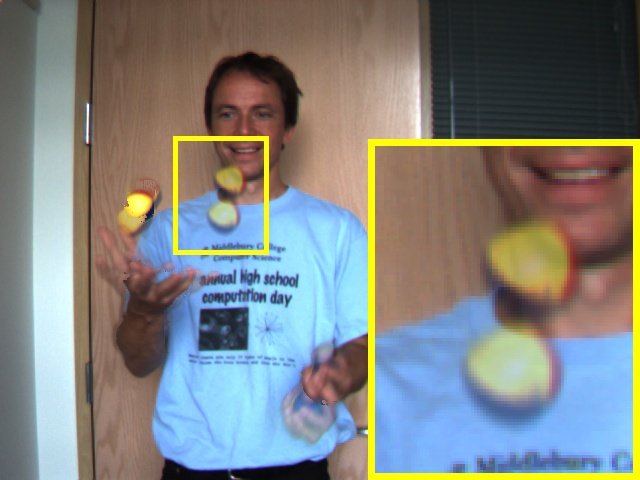}&
\includegraphics[width=0.45\linewidth]{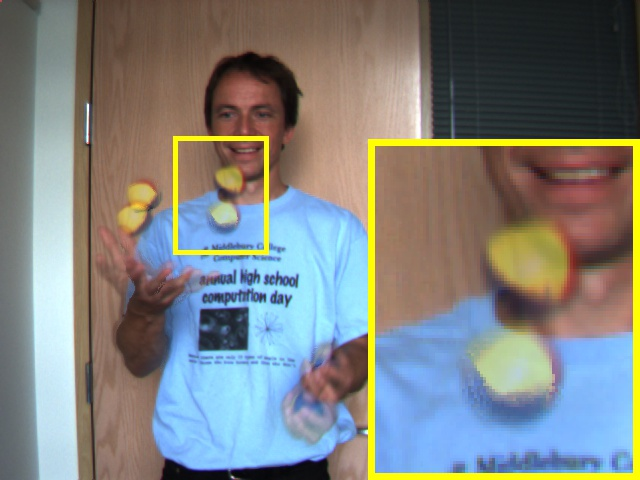}\\
			(c) EpicFlow~\cite{revaud2015epicflow}&
			(d) SPyNet~\cite{ranjan2017optical}\\

\includegraphics[width=0.45\linewidth]{supp/MiddleburySet/other-result-author/72852-lfmodel/Beanbags/frame10i11_IE1.5547_PSNR28.9425.png}&
\includegraphics[width=0.45\linewidth]{supp/MiddleburySet/other-result-author/26609-l1model/Beanbags/frame10i11_IE1.3939_PSNR30.0556.png}\\
			(e) SepConv-$L_f$~\cite{niklaus2017videoSepConv}&
			(f) SepConv-$L_1$~\cite{niklaus2017videoSepConv}\\
\includegraphics[width=0.45\linewidth]{supp/MiddleburySet/other-result-author/46043_Ours_by12661/Beanbags/frame10i11_IE1.6256_PSNR30.9598.png} &
\includegraphics[width=0.45\linewidth]{supp/MiddleburySet/other-gt-interp/Beanbags/frame10i11_IE0_PSNR48.1308.png} \\			 
			 (g) Ours &
			 (h) Ground Truth\\

		\end{tabular}
	\end{center}
	\vspace{-0.5cm}
	\caption{
	\textbf{Visual comparisons on the Middlebury~\cite{baker2011database} \textsc{Other} set.}
	%
%	The sequence is from the \textsc{Other} set.
	%
	Our method preserves the shapes of the balls well.
	}
\label{fig:MiddleburyBeanbags} %% label for entire figure
\end{figure}

\begin{figure}[t]
	%	\footnotesize
	\footnotesize
	%	\tiny
	\centering
	 % adjust horizontal space
	 % adjust vertical space
	\begin{center}
		\begin{tabular}{cc}
			\includegraphics[width=0.45\linewidth]{supp/MiddleburySet/other-result-author/MIND/MiniCooper/frame10i11_IE2.3791_PSNR27.5667.png}&
			\includegraphics[width=0.45\linewidth]{supp/MiddleburySet/other-result-author/demo_outputMB_toflow/MiniCooper/frame10i11_IE1.0796_PSNR30.5187.png}\\
			(a) MIND~\cite{long2016learning}&
			(b) ToFlow~\cite{xue2017video}\\
			
			\includegraphics[width=0.45\linewidth]{supp/MiddleburySet/other-result-author/epicflow/MiniCooper/frame10i11_IE1.328_PSNR29.4374.png}&
			\includegraphics[width=0.45\linewidth]{supp/MiddleburySet/other-result-author/spynet/MiniCooper/frame10i11_IE1.3407_PSNR29.6968.png}\\
			(c) EpicFlow~\cite{revaud2015epicflow}&
			(d) SPyNet~\cite{ranjan2017optical}\\
			
			\includegraphics[width=0.45\linewidth]{supp/MiddleburySet/other-result-author/72852-lfmodel/MiniCooper/frame10i11_IE1.0741_PSNR30.0428.png}&
			\includegraphics[width=0.45\linewidth]{supp/MiddleburySet/other-result-author/26609-l1model/MiniCooper/frame10i11_IE0.9675_PSNR30.4501.png}\\
			(e) SepConv-$L_f$~\cite{niklaus2017videoSepConv}&
			(f) SepConv-$L_1$~\cite{niklaus2017videoSepConv}\\
			\includegraphics[width=0.45\linewidth]{supp/MiddleburySet/other-result-author/46043_Ours_by12661/MiniCooper/frame10i11_IE1.0617_PSNR31.2924.png} &
			\includegraphics[width=0.45\linewidth]{supp/MiddleburySet/other-gt-interp/MiniCooper/frame10i11_IE0_PSNR48.1308.png} \\			 
			(g) Ours &
			(h) Ground Truth\\

		\end{tabular}
	\end{center}
	\vspace{-0.5cm}
	\caption{
		\textbf{Visual comparisons on the Middlebury~\cite{baker2011database} \textsc{Other} set.}
		%
%		The sequence is from the \textsc{Other} set.
		% 
		The fine structure around the shadow of the lid constructed by our method is more consistent with the ground truth than by the other approaches.
	}
	\label{fig:MiddleburyMiniCooper} %% label for entire figure
\end{figure}

\begin{figure}[t]
	%	\footnotesize
	\footnotesize
	%	\tiny
	\centering
	 % adjust horizontal space
	 % adjust vertical space
	\begin{center}
		\begin{tabular}{cc}
			\includegraphics[width=0.45\linewidth]{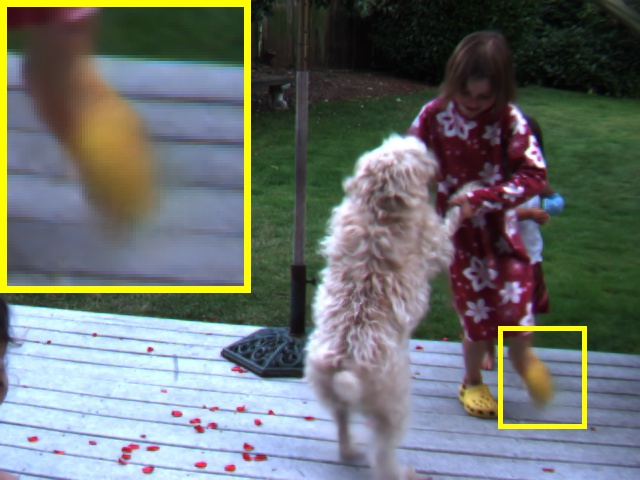}&
			\includegraphics[width=0.45\linewidth]{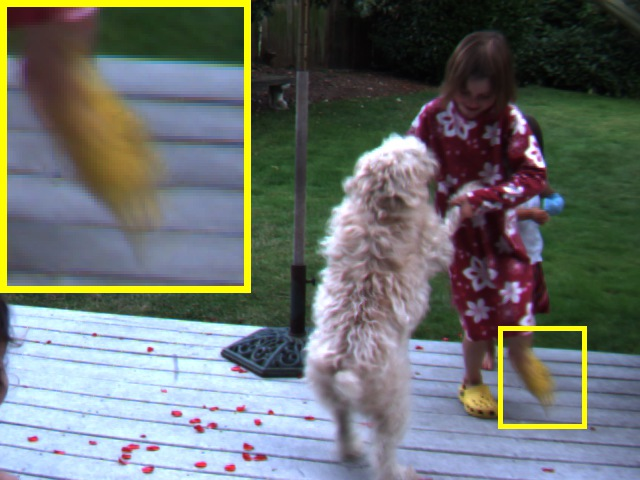}\\
			(a) MIND~\cite{long2016learning}&
			(b) ToFlow~\cite{xue2017video}\\
			
			\includegraphics[width=0.45\linewidth]{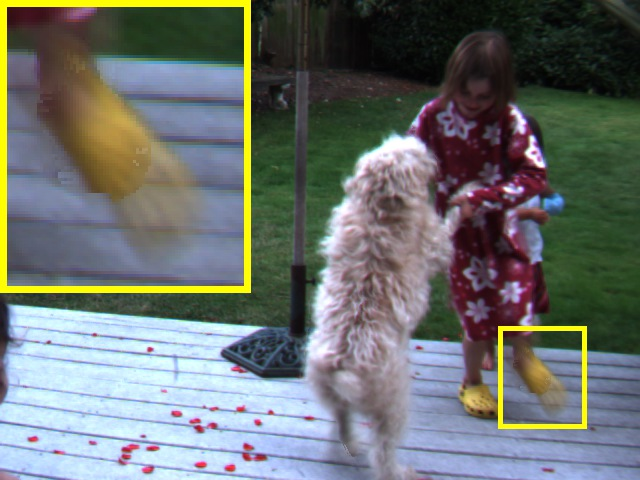}&
			\includegraphics[width=0.45\linewidth]{supp/MiddleburySet/other-result-author/spynet/DogDance/frame10i11_IE2.0234_PSNR30.467.png}\\
			(c) EpicFlow~\cite{revaud2015epicflow}&
			(d) SPyNet~\cite{ranjan2017optical}\\
			
			\includegraphics[width=0.45\linewidth]{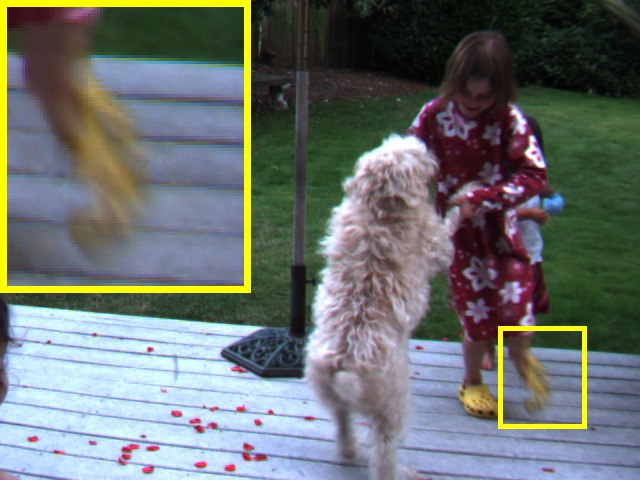}&
			\includegraphics[width=0.45\linewidth]{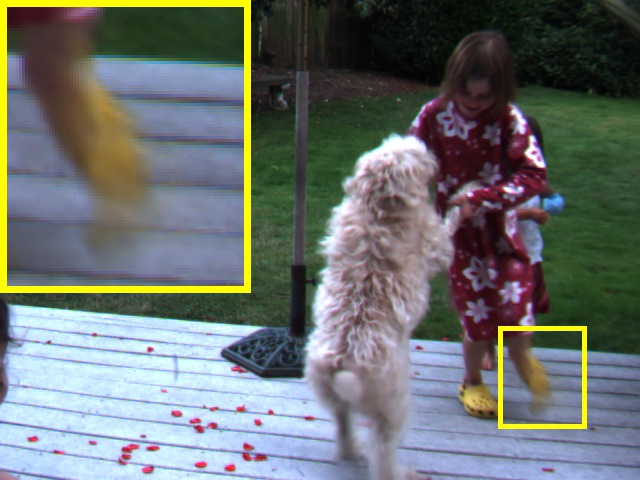}\\
			(e) SepConv-$L_f$~\cite{niklaus2017videoSepConv}&
			(f) SepConv-$L_1$~\cite{niklaus2017videoSepConv}\\
			\includegraphics[width=0.45\linewidth]{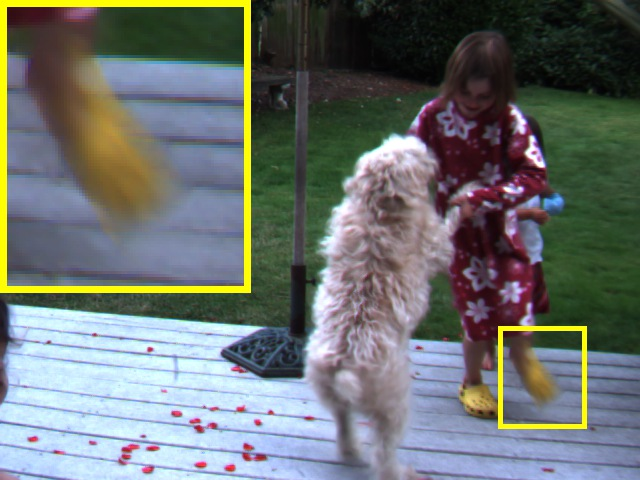} &
			\includegraphics[width=0.45\linewidth]{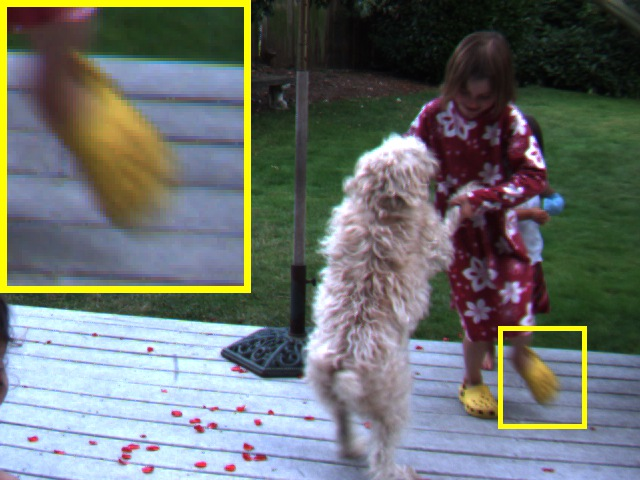} \\			 
			(g) Ours &
			(h) Ground Truth\\

		\end{tabular}
	\end{center}
	\vspace{-0.5cm}
	\caption{
		\textbf{Visual comparisons on the Middlebury~\cite{baker2011database} \textsc{Other} set.}
		%
%		The sequence is from the \textsc{Other} set.
		%
		Our method preserves the shape of the shoe well.
	}
	\label{fig:MiddleburyDogDance} %% label for entire figure
\end{figure}
