# Supplementary material for: MEMC-Net: Motion Estimation and Motion Compensation Driven Neural Network for Video Interpolation and Enhancement
Source: arXiv:1810.08768 source file (2019-09-05)
Supplement: Supplementary file 3 [file Vimeo.tex]

\begin{figure}[!h]
	%	\footnotesize
	\footnotesize
%	\tiny
	\centering
	 % adjust horizontal space
	 % adjust vertical space
\begin{center}
	\begin{tabular}{cc}
\includegraphics[width=0.49\linewidth]{supp/Vimeo90K/compare_vimeo_00065_0358/MIND/im2_IE0.84264_PSNR32.0686.png}&
\includegraphics[width=0.49\linewidth]{supp/Vimeo90K/compare_vimeo_00065_0358/toflow/out_IE0.88741_PSNR31.9207.png}\\
			(a) MIND~\cite{long2016learning}&
			(b) ToFlow~\cite{xue2017video}\\
\includegraphics[width=0.49\linewidth]{supp/Vimeo90K/compare_vimeo_00065_0358/SepConvlf/im2_IE0.90569_PSNR31.5462.png}&
\includegraphics[width=0.49\linewidth]{supp/Vimeo90K/compare_vimeo_00065_0358/SepConvl1/im2_IE0.85275_PSNR31.8495.png}\\
			(c) SepConv-$L_f$~\cite{niklaus2017videoSepConv}&
		    (d) SepConv-$L_1$~\cite{niklaus2017videoSepConv}\\
\includegraphics[width=0.49\linewidth]{supp/Vimeo90K/compare_vimeo_00065_0358/Ours/im2_IE0.99982_PSNR32.0695.png}&
\includegraphics[width=0.49\linewidth]{supp/Vimeo90K/compare_vimeo_00065_0358/GT/im2_IE0_PSNR48.1474.png} \\			 
			 (e) \Ours&
			 (f) Ground Truth\\			 
		\end{tabular}
	\end{center}
	\vspace{-0.1cm}
	\caption{
	\textbf{Visual comparisons on the Vimeo90K~\cite{xue2017video} test set. }
    Compared to existing approaches, the proposed method preserves more details near the foot.%, where quite large placement happens.
	}
\label{fig:Vimeo-00065-0358} %% label for entire figure
\end{figure}

\begin{figure}[!h]
	%	\footnotesize
	\footnotesize
	%	\tiny
	\centering
	 % adjust horizontal space
	 % adjust vertical space
	\begin{center}
		\begin{tabular}{cc}
			\includegraphics[width=0.49\linewidth]{supp/Vimeo90K/compare_vimeo_00017_0462/MIND/im2_IE0.82091_PSNR34.4151.png}&
			\includegraphics[width=0.49\linewidth]{supp/Vimeo90K/compare_vimeo_00017_0462/toflow/out_IE0.85509_PSNR34.4244.png}\\
			(a) MIND~\cite{long2016learning}&
			(b) ToFlow~\cite{xue2017video}\\
			\includegraphics[width=0.49\linewidth]{supp/Vimeo90K/compare_vimeo_00017_0462/SepConvlf/im2_IE0.90701_PSNR34.3983.png}&
			\includegraphics[width=0.49\linewidth]{supp/Vimeo90K/compare_vimeo_00017_0462/SepConvl1/im2_IE0.80952_PSNR34.7328.png}\\
			(c) SepConv-$L_f$~\cite{niklaus2017videoSepConv}&
			(d) SepConv-$L_1$~\cite{niklaus2017videoSepConv}\\
			\includegraphics[width=0.49\linewidth]{supp/Vimeo90K/compare_vimeo_00017_0462/Ours/im2_IE0.9319_PSNR34.8993.png}&
			\includegraphics[width=0.49\linewidth]{supp/Vimeo90K/compare_vimeo_00017_0462/GT/im2_IE0_PSNR48.9516.png} \\			 
			(e) \Ours &
			(f) Ground Truth\\
			
		\end{tabular}
	\end{center}
	\vspace{-0.1cm}
	\caption{
		\textbf{Visual comparisons on the Vimeo90K~\cite{xue2017video} test set. }
		Our method reconstructs the legs well.
	}
	\label{fig:Vimeo_00017_0462} %% label for entire figure
\end{figure}

\begin{figure}[!h]
	%	\footnotesize
	\footnotesize
	%	\tiny
	\centering
	 % adjust horizontal space
	 % adjust vertical space
	\begin{center}
		\begin{tabular}{cc}
			\includegraphics[width=0.49\linewidth]{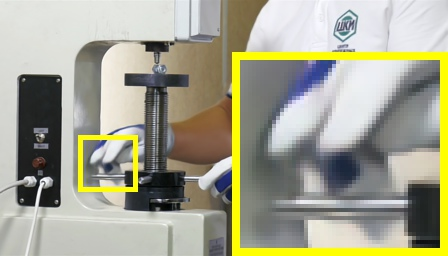}&
			\includegraphics[width=0.49\linewidth]{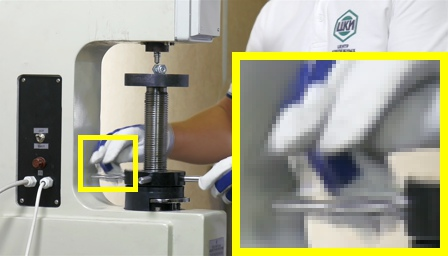}\\
			(a) MIND~\cite{long2016learning}&
			(b) ToFlow~\cite{xue2017video}\\
			\includegraphics[width=0.49\linewidth]{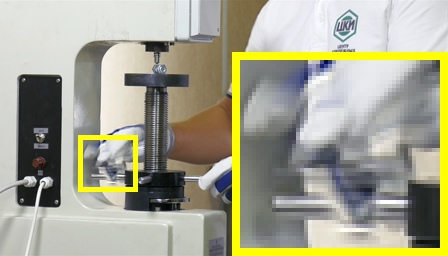}&
			\includegraphics[width=0.49\linewidth]{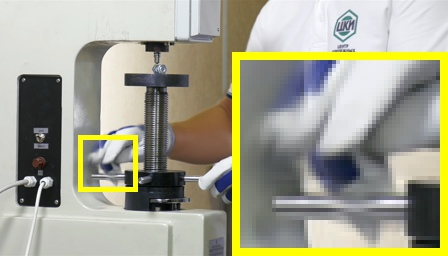}\\
			(c) SepConv-$L_f$~\cite{niklaus2017videoSepConv}&
			(d) SepConv-$L_1$~\cite{niklaus2017videoSepConv}\\
			\includegraphics[width=0.49\linewidth]{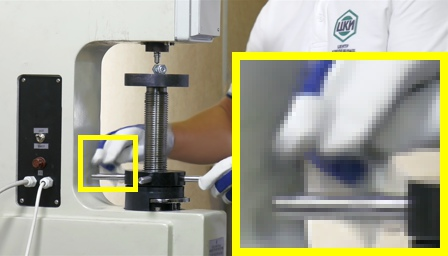}&
			\includegraphics[width=0.49\linewidth]{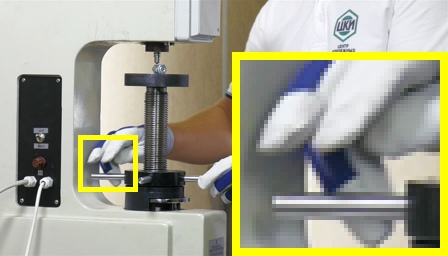} \\			 
			(e) \Ours&
			(f) Ground Truth\\
			
		\end{tabular}
	\end{center}
	\vspace{-0.1cm}
	\caption{
		\textbf{Visual comparisons on the Vimeo90K~\cite{xue2017video} test set. }
		Our method maintains the structures of both the fingers in gloves and the steel bar of the devices well.
	}
	\label{fig:Vimeo_00041_0001} %% label for entire figure
\end{figure}

\begin{figure}[!h]
	%	\footnotesize
	\footnotesize
	%	\tiny
	\centering
	 % adjust horizontal space
	 % adjust vertical space
	\begin{center}
		\begin{tabular}{cc}
			\includegraphics[width=0.49\linewidth]{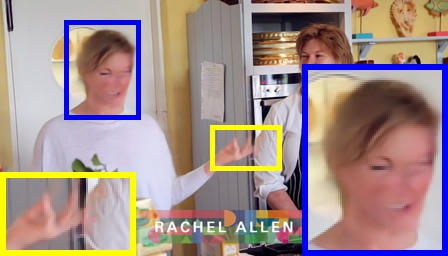}&
			\includegraphics[width=0.49\linewidth]{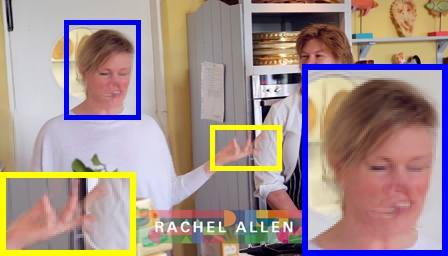}\\
			(a) MIND~\cite{long2016learning}&
			(b) ToFlow~\cite{xue2017video}\\
			\includegraphics[width=0.49\linewidth]{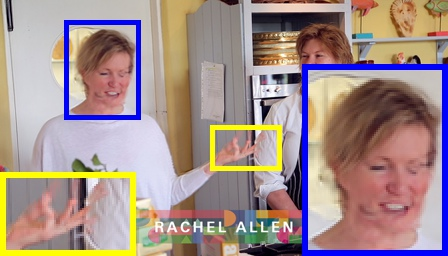}&
			\includegraphics[width=0.49\linewidth]{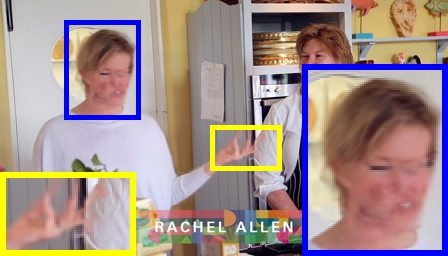}\\
			(c) SepConv-$L_f$~\cite{niklaus2017videoSepConv}&
			(d) SepConv-$L_1$~\cite{niklaus2017videoSepConv}\\
			\includegraphics[width=0.49\linewidth]{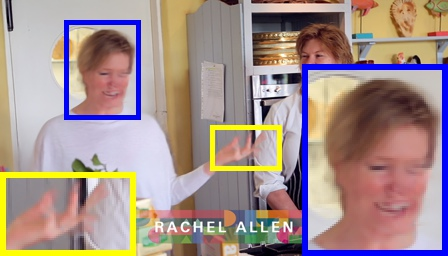}&
			\includegraphics[width=0.49\linewidth]{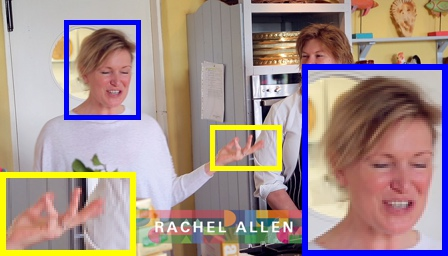} \\			 
			(e) \Ours &
			(f) Ground Truth\\
			
		\end{tabular}
	\end{center}
	\vspace{-0.1cm}
	\caption{
		\textbf{Visual comparisons on the Vimeo90K~\cite{xue2017video} test set. }
		The proposed method maintains the shape of the face well, while existing approaches distort the face.
	}
	\label{fig:Vimeo_00066_0074} %% label for entire figure
\end{figure}
