# Supplementary material for: MEMC-Net: Motion Estimation and Motion Compensation Driven Neural Network for Video Interpolation and Enhancement
Source: arXiv:1810.08768 source file (2019-09-05)
Supplement: Supplementary file 4 [file UCF101.tex]

\begin{figure}[!h]
	%	\footnotesize
	\footnotesize
%	\tiny
	\centering
	 % adjust horizontal space
	 % adjust vertical space
\begin{center}
	\begin{tabular}{cc}
\includegraphics[width=0.49\linewidth]{supp/MiddleburySet/eval-result-author/67599_overlay/Dumptruck/frame10i11.png}&
\includegraphics[width=0.49\linewidth]{supp/MiddleburySet/eval-result-author/epicflow/Dumptruck/frame10i11.png}\\
			(a) Overlay&
			(b) EpicFlow~\cite{revaud2015epicflow}\\
\includegraphics[width=0.49\linewidth]{supp/MiddleburySet/eval-result-author/spynet/Dumptruck/frame10i11.png}&
\includegraphics[width=0.49\linewidth]{supp/MiddleburySet/eval-result-author/33758-lf/Dumptruck/frame10i11.png}\\
			(c) SPyNet~\cite{ranjan2017optical}&
			(d) SepConv-$L_f$~\cite{niklaus2017videoSepConv}\\
\includegraphics[width=0.49\linewidth]{supp/MiddleburySet/eval-result-author/93785-l1/Dumptruck/frame10i11.png}&
\includegraphics[width=0.49\linewidth]{supp/MiddleburySet/eval-result-author/46043_Ours_by12661/Dumptruck/frame10i11.png} \\			 
			 (e) SepConv-$L_1$~\cite{niklaus2017videoSepConv}&
			 (f) FGIK\\
		\end{tabular}
	\end{center}
% \vspace{-0.1cm}
	\caption{
	\textbf{Visual comparisons on UCF101~\cite{soomro2012ucf101}. }
	The sequence is from the \textsc{Evaluation} set.
	}
\label{fig:UCF101-} %% label for entire figure
\end{figure}
